# Supplementary material for: Nuance Matters: Probing Epistemic Consistency in Causal Reasoning
Source: arXiv:2409.00103 source file (2024-08-27)
Supplement: Supplementary file 2 [file open-source.tex]

\subsection{Generation}
In zero-shot settings, open-source models often struggle to produce text in a specific format consistently. This inconsistency requires steering the models towards generating easily extractable text using the same set of rules each time (e.g., find the lines that start with '1.' or '2.').
\subsection{Ranking}
Similarly, we provide separate scripts for the ranking component. In this part, the models rank the 10 arguments in different ways. For instance, some models output the ranking on a single line, while others insert a line break between each number. Therefore, the primary challenge lies in extracting the ranking correctly.
