# Supplementary material for: Nuance Matters: Probing Epistemic Consistency in Causal Reasoning
Source: arXiv:2409.00103 source file (2024-08-27)
Supplement: Supplementary file 3 [file appendix_metrics.tex]

\setlength{\columnsep}{2.0cm}

\begin{tabular}{l|p{\columnsep}p{\columnsep}p{\columnsep}|C{\columnsep}|C{\columnsep}}
\toprule 
Aspect & \multicolumn{3}{>{\columncolor{\rankingColor}}m{6.8cm}}{\centering \textit{Pairwise ranking concordance}} 
& \multicolumn{1}{>{\columncolor{\crossColor}}m{2.0cm}}{\textit{Cross-group position}} 
& \multicolumn{1}{>{\columncolor{\clusteringColor}}m{2.0cm}}{\textit{Intra-group clustering}} 
% & \multicolumn{1}{>{\columncolor{\clusteringColor}}}{\textit{Intra-group clustering}} 
\\
    \midrule
    & \tauA$\uparrow$ & \tauD$\uparrow$ & \tauOverall$\uparrow$ & \centering \CGP $\uparrow$ &  \multicolumn{1}{>{\columncolor{white}}c}{\IGC $\uparrow$} \\
    \midrule
    \multicolumn{6}{>{\columncolor{mygray}}c}{\textit{Closed-Source Models}}\\ \midgrayline

    % full generation
    GPT-3.5 Turbo & 0.065 \stdvalue{0.417} & 0.101 \stdvalue{0.412} & 0.233 \stdvalue{0.288} & 0.677 \stdvalue{0.228} & 0.563 \stdvalue{0.198} \\
    GPT-4 & 0.306 \stdvalue{0.437} & 0.075 \stdvalue{0.434} & 0.567 \stdvalue{0.201} & 0.934 \stdvalue{0.119} & 0.836 \stdvalue{0.219} \\
    GPT-4 Turbo & \textbf{0.381 \stdvalue{0.432}} & 0.098 \stdvalue{0.431} & 0.535 \stdvalue{0.319} & 0.886 \stdvalue{0.233} & 0.842 \stdvalue{0.217} \\
    GPT-4o mini & 0.168 \stdvalue{0.417} & 0.057 \stdvalue{0.369} & 0.474 \stdvalue{0.240} & 0.882 \stdvalue{0.192} & 0.780 \stdvalue{0.239} \\
    GPT-4o & 0.193 \stdvalue{0.447} & 0.112 \stdvalue{0.413} & 0.606 \stdvalue{0.157} & \textbf{0.984 \stdvalue{0.071}} & \textbf{0.962 \stdvalue{0.123}} \\

    \midgrayline

    Claude 3 Haiku & 0.152 \stdvalue{0.408} & 0.072 \stdvalue{0.394} & 0.450 \stdvalue{0.286} & 0.860 \stdvalue{0.229} & 0.813 \stdvalue{0.241} \\
    Claude 3 Sonnet & 0.212 \stdvalue{0.432} & 0.122 \stdvalue{0.429} & 0.494 \stdvalue{0.290} & 0.878 \stdvalue{0.219} & 0.825 \stdvalue{0.242} \\
    Claude 3 Opus & 0.363 \stdvalue{0.448} & 0.214 \stdvalue{0.482} & 0.535 \stdvalue{0.405} & 0.866 \stdvalue{0.282} & 0.881 \stdvalue{0.204} \\
    Claude 3.5 Sonnet & 0.310 \stdvalue{0.411} & \textbf{0.304 \stdvalue{0.443}} & \textbf{0.652 \stdvalue{0.202}} & 0.964 \stdvalue{0.118} & 0.929 \stdvalue{0.164} \\

    \midgrayline

    Gemini 1.5 Flash & 0.229 \stdvalue{0.402} & 0.115 \stdvalue{0.385} & 0.398 \stdvalue{0.257} & 0.790 \stdvalue{0.203} & 0.641 \stdvalue{0.231} \\
    Gemini 1.5 Pro & 0.332 \stdvalue{0.358} & 0.049 \stdvalue{0.378} & 0.539 \stdvalue{0.191} & 0.909 \stdvalue{0.137} & 0.792 \stdvalue{0.237} \\

  \bottomrule
\end{tabular}
