# Supplementary material for: Nuance Matters: Probing Epistemic Consistency in Causal Reasoning
Source: arXiv:2409.00103 source file (2024-08-27)
Supplement: Supplementary file 4 [file checklist.tex]

This paper:
\begin{itemize}
    \item Includes a conceptual outline and/or pseudocode description of AI methods introduced (yes/partial/no/NA) yes
    \item Clearly delineates statements that are opinions, hypothesis, and speculation from objective facts and results (yes/no) yes
    \item Provides well marked pedagogical references for less-familiare readers to gain background necessary to replicate the paper (yes/no) yes

\end{itemize}



\noindent Does this paper make theoretical contributions? (yes/no) yes
\begin{itemize}
    \item All assumptions and restrictions are stated clearly and formally. (yes/partial/no) yes
    \item All novel claims are stated formally (e.g., in theorem statements). (yes/partial/no) yes
    \item Proofs of all novel claims are included. (yes/partial/no) yes
    \item Proof sketches or intuitions are given for complex and/or novel results. (yes/partial/no) yes
    \item Appropriate citations to theoretical tools used are given. (yes/partial/no) yes
    \item All theoretical claims are demonstrated empirically to hold. (yes/partial/no/NA) yes
    \item All experimental code used to eliminate or disprove claims is included. (yes/no/NA) yes
\end{itemize}


\noindent Does this paper rely on one or more datasets? (yes/no) yes

\begin{itemize}
    \item A motivation is given for why the experiments are conducted on the selected datasets (yes/partial/no/NA) yes
    \item All novel datasets introduced in this paper are included in a data appendix. (yes/partial/no/NA) yes
    \item All novel datasets introduced in this paper will be made publicly available upon publication of the paper with a license that allows free usage for research purposes. (yes/partial/no/NA) yes
    \item All datasets drawn from the existing literature (potentially including authors’ own previously published work) are accompanied by appropriate citations. (yes/no/NA) yes
    \item All datasets drawn from the existing literature (potentially including authors’ own previously published work) are publicly available. (yes/partial/no/NA) yes
    \item All datasets that are not publicly available are described in detail, with explanation why publicly available alternatives are not scientifically satisficing. (yes/partial/no/NA) yes
\end{itemize}

\noindent Does this paper include computational experiments? (yes/no) yes

\begin{itemize}
    \item Any code required for pre-processing data is included in the appendix. (yes/partial/no) yes
    \item All source code required for conducting and analyzing the experiments is included in a code appendix. (yes/partial/no) yes
    \item All source code required for conducting and analyzing the experiments will be made publicly available upon publication of the paper with a license that allows free usage for research purposes. (yes/partial/no) yes
    \item All source code implementing new methods have comments detailing the implementation, with references to the paper where each step comes from (yes/partial/no) yes
    \item If an algorithm depends on randomness, then the method used for setting seeds is described in a way sufficient to allow replication of results. (yes/partial/no/NA) yes
    \item This paper specifies the computing infrastructure used for running experiments (hardware and software), including GPU/CPU models; amount of memory; operating system; names and versions of relevant software libraries and frameworks. (yes/partial/no) yes
    \item This paper formally describes evaluation metrics used and explains the motivation for choosing these metrics. (yes/partial/no) yes
    \item This paper states the number of algorithm runs used to compute each reported result. (yes/no) yes
    \item Analysis of experiments goes beyond single-dimensional summaries of performance (e.g., average; median) to include measures of variation, confidence, or other distributional information. (yes/no) yes
    \item The significance of any improvement or decrease in performance is judged using appropriate statistical tests (e.g., Wilcoxon signed-rank). (yes/partial/no) yes
    \item This paper lists all final (hyper-)parameters used for each model/algorithm in the paper’s experiments. (yes/partial/no/NA) yes
    \item This paper states the number and range of values tried per (hyper-) parameter during development of the paper, along with the criterion used for selecting the final parameter setting. (yes/partial/no/NA) yes
\end{itemize}
